# Supplementary material for: Geometries, interaction energies and bonding in [Po(H$_2$O)$_n$]$^{4+}$ and [PoCl$_n$]$^{4-n}$ complexes
Source: arXiv:2208.13570 source file (2022-09-30)
Supplement: Supplementary file 1 [file SI.pdf]

# Supporting Information for "Geometries, interaction energies and bonding in $[Po(H_2O)_n]^{4+}$ and $[PoCl_n]^{4-n}$ complexes", by Zhutova *et al.*

Date of preparation: August 29, 2022

Table S1 Interaction energies ($kcal\,mol^{-1}$) with BSSE correction obtained at various levels of theory for polonium(IV) complexes with water, computed according to Eqs. 1 and 2 (see main text).

| $n(H_2O)$ | CCSD(T) / aug-cc-pVDZ | MP2 / aug-cc-pVDZ | MP2 / aug-cc-pVTZ | MP2 / aug-cc-pVQZ* | MP2 / def2-TZVP | MP2 / def2-QZVP |
|---|---|---|---|---|---|---|
| 1 | −236.2 | −249.2 | −257.9 | −262.7 | −262.0 | −263.8 |
| 2 | −409.5 | −439.0 | −454.7 | −462.9 | −461.4 | −464.9 |
| 3 | −541.1 | −586.4 | −607.7 | −618.5 | −616.1 | −621.4 |
| 4 | | −694.9 | −718.8 | | −728.9 | |
| 5 | | −791.8 | −817.6 | | −829.4 | |
| 6 | | −875.8 | −903.1 | | −918.2 | |
| 7 | | −941.2 | −971.1 | | −987.8 | |
| 8 | | −1004.4 | −1035.9 | | −1054.0 | |
| 9 | | −1052.7 | −1085.5 | | −1104.4 | |

*Geometries for these calculations were taken from the MP2/aug-cc-pVTZ structures (single points).

Table S2 Interaction energies ($kcal\,mol^{-1}$) without BSSE correction obtained at various levels of theory for polonium(IV) complexes with water, computed according to Eq. 1 (see main text).

| $n(H_2O)$ | CCSD(T) / aug-cc-pVDZ | CCSD(T) / aug-cc-pVTZ | CCSD(T) / def2-TZVP | MP2 / aug-cc-pVDZ | MP2 / aug-cc-pVTZ | MP2 / aug-cc-pVQZ* | MP2 / def2-TZVP | MP2 / def2-QZVP |
|---|---|---|---|---|---|---|---|---|
| 1 | −238.6 | −254.6 | −247.4 | −251.7 | −261.0 | −267.8 | −264.7 | −262.5 |
| 2 | −414.3 | −446.2 | −431.0 | −443.7 | −460.8 | −472.4 | −466.8 | −462.3 |
| 3 | −548.2 | | | −593.1 | −616.6 | −632.0 | −624.6 | −617.6 |
| 4 | | | | −703.0 | −730.0 | | −739.9 | |
| 5 | | | | −801.1 | −830.9 | | −843.1 | |
| 6 | | | | −886.1 | −917.9 | | −934.9 | |
| 7 | | | | −952.4 | −987.6 | | −1006.2 | |
| 8 | | | | −1016.4 | −1054.6 | | −1074.0 | |
| 9 | | | | −1065.4 | −1106.5 | | −1126.0 | |

*Geometries for these calculations were taken from the MP2/aug-cc-pVTZ structures (single points).

Table S3 Interaction energies ($kcal\,mol^{-1}$) with BSSE correction obtained at the MP2 level of theory with various basis sets for polonium(IV) complexes with chlorides, computed according to Eqs. 1 and 2 (see main text).

| $n(Cl^-)$ | aug-cc-pVDZ | aug-cc-pVTZ | aug-cc-pVQZ* | def2-TZVP | def2-QZVP* |
|---|---|---|---|---|---|
| 1 | −859.8 | −877.4 | −884.4 | −883.7 | −885.5 |
| 2 | −1371.5 | −1403.4 | −1414.8 | −1415.0 | −1416.7 |
| 3 | −1693.1 | −1734.0 | −1748.4 | −1749.2 | −1750.1 |
| 4 | −1847.0 | −1889.0 | −1905.6 | −1911.4 | −1909.3 |
| 5 | −1897.8 | | | −1974.3 | −1972.5 |
| 6 | −1886.5 | | | −1947.8 | −1949.5 |
| 7 | −1749.1 | | | −1861.4 | −1809.6 |
| 8 | −1546.5 | | | −1650.3 | −1601.8 |

*Geometries for these calculations were taken from the MP2/aug-cc-pVTZ and MP2/def2-TZVP structures, respectively (single points).

Table S4 Interaction energies (kcal mol$^{-1}$) without BSSE correction obtained at the MP2 level of theory with various basis sets for polonium(IV) complexes with chlorides, computed according to Eq. 1 (see main text).

| $n(Cl^-)$ | aug-cc-pVDZ | aug-cc-pVTZ | aug-cc-pVQZ* | def2-TZVP | def2-QZVP* |
|---|---|---|---|---|---|
| 1 | −862.0 | −880.0 | −887.7 | −888.9 | −887.8 |
| 2 | −1376.1 | −1408.6 | −1421.2 | −1425.2 | −1421.9 |
| 3 | −1700.3 | −1742.3 | −1758.0 | −1765.4 | −1759.0 |
| 4 | −1857.6 | −1899.5 | −1916.8 | −1933.0 | −1923.2 |
| 5 | −1923.0 | | | −2003.0 | −1990.9 |
| 6 | −1905.1 | | | −1986.1 | −1972.7 |
| 7 | −1772.9 | | | −1904.5 | −1837.9 |
| 8 | −1575.7 | | | −1696.8 | −1634.1 |

*Geometries for these calculations were taken from the MP2/aug-cc-pVTZ and MP2/def2-TZVP structures, respectively (single points).

Table S5 Mean MP2 Po−O bond lengths (Å), obtained for polonium(IV) complexes with water for various basis sets.

| $n(H_2O)$ | aug-cc-pVDZ | aug-cc-pVTZ | def2-TZVP | def2-QZVP |
|---|---|---|---|---|
| 1 | 2.08 | 2.04 | 2.03 | 2.02 |
| 2 | 2.11 | 2.08 | 2.07 | 2.06 |
| 3 | 2.15 | 2.11 | 2.11 | 2.10 |
| 4 | 2.20 | 2.17 | 2.17 | 2.16 |
| 5 | 2.25 | 2.22 | 2.22 | 2.21 |
| 6 | 2.30 | 2.27 | 2.27 | 2.26 |
| 7 | 2.34 | 2.31 | 2.31 | 2.30 |
| 8 | 2.37 | 2.34 | 2.34 | 2.34 |
| 9 | 2.41 | 2.38 | 2.39 | 2.37 |

Table S6 Mean MP2 Po−O bond lengths (Å), obtained for polonium(IV) complexes with chlorides for various basis sets

| $n(Cl^-)$ | aug-cc-pVDZ | aug-cc-pVTZ | def2-TZVP |
|---|---|---|---|
| 1 | 2.30 | 2.25 | 2.25 |
| 2 | 2.33 | 2.29 | 2.28 |
| 3 | 2.40 | 2.35 | 2.34 |
| 4 | 2.52 | 2.48 | 2.47 |
| 5 | 2.59 | | 2.54 |
| 6 | 2.66 | | 2.60 |
| 7 | 2.77 | | 2.72 |
| 8 | 2.88 | | 2.83 |

Table S7 MP2/def2-TZVP atomic charges for polonium(IV) complexes with chlorides derived from different charge schemes.

| Molecule | QTAIM | | | Mulliken | | | Hirshfeld | | |
|---|---|---|---|---|---|---|---|---|---|
| | q(Po) | q(Cl) | | q(Po) | q(Cl) | | q(Po) | q(Cl) | |
| $[PoCl]^{3+}$ | 2.52 | 0.48 | | 2.23 | 0.77 | | 2.15 | 0.85 | |
| $[PoCl_2]^{2+}$ | 2.06 | −0.03 | | 1.52 | 0.24 | | 1.34 | 0.33 | |
| $[PoCl_3]^{+}$ | 1.94 | −0.31 | | 1.25 | −0.08 | | 0.93 | 0.02 | |
| $PoCl_4$ | 1.98 | −0.50 | | 1.25 | −0.31 | | 0.77 | −0.19 | |
| $[PoCl_5]^{-}$ | 2.06 | −0.64 | (x2) | 1.29 | −0.49 | (x2) | 0.71 | −0.40 | (x2) |
| | | −0.59 | (x3) | | −0.43 | (x3) | | −0.34 | (x3) |
| $[PoCl_6]^{2-}$ | 2.13 | −0.69 | | 1.43 | −0.57 | | 0.67 | −0.44 | |
| $[PoCl_7]^{3-}$ | 2.13 | −0.74 | (x5) | 1.84 | −0.70 | (x5) | 0.92 | −0.58 | (x5) |
| | | −0.71 | (x2) | | −0.67 | (x2) | | −0.50 | (x2) |
| $[PoCl_8]^{4-}$ | 2.12 | −0.76 | | 1.96 | −0.74 | | 1.02 | −0.63 | |
